# Supplementary material for: Provable Filter Pruning for Efficient Neural Networks
Source: arXiv:1911.07412 source file (2020-03-23)
Supplement: Supplementary file 1 [file problem-definition.tex]

\section{Problem Definition}
\label{sec:problem-definition}

The set of parameters $\theta$ of a CNN with $L$ convolutional layers is a tuple of 4-dimensional weight matrices corresponding to each layer, i.e., $\theta = (\WW^1, \ldots, \WW^L)$. The set of parameters $\theta$ defines the mapping $f_\theta: \XX \to \YY$ from the input space $\XX$ to the output space $\YY$. We consider the setting where a neural network $\f(\cdot)$ has been trained on a training set of independent and identically distributed (i.i.d.) samples from a joint distribution defined on $\XX \times \YY$, 
yielding parameters $\param$. We let $\DD$ denote the marginal distribution over the input space $\XX$ and define the size of the parameter tuple $\param$, $\size{\param}$, to be the number of all non-zero entries in the weight tensors $\WW^1,\ldots,\WW^L$.

For any given $\epsilon, \delta \in (0,1)$, our overarching goal is to use a randomized algorithm to generate a sparse reparameterization $\paramHat$ of $\theta$ such that $\size{\paramHat} \ll \size{\param}$ and for $\Point \sim \DD$ the reference network output $\f(\Input)$ can be approximated by $\fHat(\Input)$ up to $1 \pm \eps$ entry-wise\footnote{For two tensors $T_1, T_2$ of same dimensions, $T_1 \in (1 \pm \epsilon) T_2$ denotes follow entry-wise bound: for each scalar entry $t_1$ in tensor $T_1$,  $t_1 \in (1 \pm \epsilon) t_2$, where $t_2$ is the corresponding entry in $T_2$.} multiplicative error with probability greater than $1- \delta$. \CB{TODO: Define what $\size{\cdot}$ means}

\CB{TODO: Formal but simple problem definition based on FNNs}
\begin{definition}[$(\epsilon, \delta)$-coreset]
For $\eps, \delta \in (0,1)$, and a set of parameters $\param = \paramDef$, $\paramHat = \paramHatDef$ such that $\size{\paramHat} \ll \size{\param}$, is an $(\eps, \delta)$-coreset for the original set of parameters $\theta$ if 
$$
\Pr_{\paramHat, \Point} (\fHat (\Input) \in (1 \pm \eps) \f(\Input)) \ge 1 - \delta,
$$
where $\Pr_{\paramHat, \Point}$ denotes the probability measure with respect to a random data point $\Point \sim \DD$ and the output $\paramHat$ generated by a randomized compression scheme.
\end{definition}
